# Supplementary material for: A Probabilistic Model of Activity Recognition with Loose Clothing
Source: arXiv:2209.11579 source file (2022-09-23)
Supplement: Supplementary file 1 [file appendix.tex]

\subsection{Simulation of scotch yoke}\label{s:prob}
\subsubsection{The \gls{pdf} of fabric position}\label{s:pdf}
The following equations are \gls{pdf} of mass position $\Xr$ \cite{shin2008fundamentals} and additional information $\xf$. 
\begin{equation}
f(\xr)=
\begin{cases}
\frac{1}{\pi\sqrt{1-\xr^2}}& \text{$-1<\xr<1$}\\
0& \text{otherwise}\\
\end{cases}
\end{equation}

\begin{equation}
f(\Xd)=
\begin{cases}
\frac{1}{2\v L}& \text{$-\v L<\Xd<\v L$}\\
0& \text{otherwise}\\
\end{cases}
\end{equation}
Find \gls{pdf} of $\xr + \Xd$. Range of $\xf = \xr + \Xd$ is $[-1-\v L,1+\v L]$.
The density function for the sum is given by \cite{dominguez2015history}
\begin{equation}
f_{(\xr + \Xd)}(\xf)= f(\xr)*f(\Xd) =  \int_{-\infty}^{+\infty}f_{\xr}(\xr)f_{\xr}(\xf-\xr)\,d(\xr)
\end{equation}

Thus,
\begin{equation}
\begin{split}
f_{\xr+\Xd}(\xf)&= (f(\xr)*\Xd))(\xf) = \int_{-\infty}^{+\infty}\frac{1}{\pi\sqrt{1-\xr^2}} \frac{1}{2\v L}\,d(\xr)\\
& = \int_{-\infty}^{+\infty}\frac{1}{\pi\sqrt{1-\xr^2 }} \frac{1}{2\v L}\,d(\xr)\\
&=  \frac{1}{2\v L \pi} \int_{-\infty}^{+\infty}\frac{1}{\sqrt{1-\xr^2 }}\,d(\xr)\\
&=\frac{1}{2\v L \pi}(sin^{-1}(\xr) + c)
\end{split}
\label{pdf:fabric}
\end{equation}


%(a) 
%$\v L\geq1$,
%$-1-\v L<T<1-\v L$
%\begin{equation}
%\begin{split}
%f_{X+Y}(T)&=\frac{1}{2\v L \pi}(sin^{-1}(X) + c)\bigg|^{T+\v L}_{-1}\\
%&= \frac{1}{2\v L \pi}(sin^{-1}(T+\v L)+\frac{\pi}{2}) \\
%\end{split}
%\end{equation}

%$1-\v L \leq T \leq -1+\v L$
%\begin{equation}
%\begin{split}
%f_{X+Y}(T)&=\frac{1}{2\v L \pi}(sin^{-1}(X) + c)\bigg|^{1}_{-1}\\
%&= \frac{1}{2\v L}\\
%\end{split}
%\end{equation}

%$-1+\v L<T<\v L+1$
%\begin{equation}
%\begin{split}
%f_{X+Y}(T)&=\frac{1}{2\v L \pi}(sin^{-1}(X) + c)\bigg|^{1}_{T-\v L}\\
%&= \frac{1}{2\v L \pi}(-sin^{-1}(T-\v L)+\frac{\pi}{2}) \\
%\end{split}
%\end{equation}

%(b) 
%$0<\v L<1$,
$-1-\v L\leq \xf <-1+\v L$
\begin{equation}
\begin{split}
f(\xf)&=\frac{1}{2\v L \pi}(sin^{-1}(\xr) + c)\bigg|^{\xf+\v L}_{-1}\\
&= \frac{1}{2\v L \pi}(sin^{-1}(\xf+\v L)+\frac{\pi}{2}) \\
\end{split}
\end{equation}

$-1+ \v L \leq  \xf \leq 1-\v L$
\begin{equation}
\begin{split}
f(\xf)&=  \frac{1}{2\v L \pi}(sin^{-1}(\xr) + c)\bigg|^{\v L+\xf}_{-\v L+\xf}\\
&= \frac{1}{2\v L \pi}(sin^{-1}(\xf+\v L)-sin^{-1}(\xf-\v L))
\end{split}
\end{equation}

$1-\v L < \xf \leq \v L+1$
\begin{equation}
\begin{split}
f(\xf)&=\frac{1}{2\v L \pi}(sin^{-1}(\xr) + c)\bigg|^{1}_{\xf-\v L}\\
&= \frac{1}{2\v L \pi}(-sin^{-1}(\xf-\v L)+\frac{\pi}{2}) \\
&= \frac{1}{2\v L \pi}(sin^{-1}(-\xf+\v L)+\frac{\pi}{2}) \\
\end{split}
\end{equation}

In summary, the \gls{pdf} of fabric position $\Xf$ is: 
\begin{equation}
f(\xf)=
\begin{cases}
\frac{sin^{-1}(\xf+\v L)+\frac{\pi}{2}}{2\v L \pi}& \text{$-1-\v L\leq \xf <-1+\v L$}\\
\frac{sin^{-1}(\xf+\v L)-sin^{-1}(\xf-\v L)}{2\v L \pi}& \text{$-1+ \v L \leq  \xf \leq 1-\v L$}\\
\frac{sin^{-1}(-\xf+\v L)+\frac{\pi}{2}}{2\v L \pi}& \text{$1-\v L < \xf \leq \v L+1$
}\\
0& \text{otherwise}\\
\end{cases}
\end{equation}

\subsubsection{The \gls{cdf} of fabric position}\label{s:cdf}
Find \gls{cdf} of $\xr + \Xd$, we compute $F(\xf)$ using $f(\xf)$.  

$-1-\v L\leq \xf <-1+\v L$
\begin{equation}
\begin{split}
&F(\xf)=\int_{-1-\v L}^{\xf}\frac{sin^{-1}(\xf+\v L)+\frac{\pi}{2}}{2\v L \pi}\,d(\xf)\\
&=\frac{\sqrt{-(\xf+\v L)^2+1}+(\xf+\v L)sin^{-1}(\v L+\xf)+\frac{\pi \xf}{2}}{2\v L \pi}\bigg|^{\xf}_{-1-\v L}\\
&= \frac{\pi(\v L +\xf)+2\sqrt{-(\v L + \xf )^2 +1}}{4\v L \pi}\\
&+\frac{2(\v L +\xf)sin^{-1}(\v L+\xf)}{4\v L \pi}
\end{split}
\end{equation}

$-1+ \v L \leq  \xf \leq 1-\v L$
\begin{equation}
\begin{split}
&F(\xf)=\int_{-1-\v L}^{-1+\v L}\frac{sin^{-1}(\xf+\v L)+\frac{\pi}{2}}{2\v L \pi}\,d(\xf)\\
&+\int_{-1+\v L}^{\xf}\frac{sin^{-1}(\xf+\v L)-sin^{-1}(\xf-\v L)}{2\v L \pi}\,d(\xf)\\
&=\frac{\pi(\v L-\frac{1}{2})+2\sqrt{-(\v L-1)\v L}+(1-2\v L)sin^{-1}(1-2\v L)}{2\v L \pi}\\
&+\frac{\sqrt{-(\xf+\v L)^2+1}-\sqrt{-(\xf-\v L)^2+1}}{2\v L \pi}\bigg|^{\xf}_{-1+\v L}\\
&+\frac{(\xf-\v L)sin^{-1}(\v L -\xf)+(\v L+\xf)sin^{-1}(\xf+\v L)}{2\v L \pi}\bigg|^{\xf}_{-1+\v L}\\
&=\frac{\pi\v L +\sqrt{-(\xf+\v L)^2+1}-\sqrt{-(\xf-\v L)^2+1}}{2\v L \pi}\\
&+\frac{(\xf-\v L)sin^{-1}(\v L -\xf)+(\v L+\xf)sin^{-1}(\xf+\v L)}{2\v L \pi}\\
\end{split}
\end{equation}

$1-\v L < \xf \leq \v L+1$
\begin{equation}
\begin{split}
&F(\xf)=\int_{-1-\v L}^{-1+\v L}\frac{sin^{-1}(\xf+\v L)+\frac{\pi}{2}}{2\v L \pi}\,d(\xf)\\
&+\int_{-1+\v L}^{1-\v L}\frac{sin^{-1}(\xf+\v L)-sin^{-1}(\xf-\v L)}{2\v L \pi}\,d(\xf)\\
&+\int_{1-\v L}^{\xf}\frac{1}{2\v L \pi}(sin^{-1}(-\xf+\v L)+\frac{\pi}{2})\,d(\xf)\\
&=\frac{\pi(\v L-\frac{1}{2})+2\sqrt{-(\v L-1)\v L}+(1-2\v L)sin^{-1}(1-2\v L)}{2\v L \pi}\\
&+\frac{-2\sqrt{-(2\v L-1)^2+1}+\pi+(2-4\v L)sin^{-1}(2\v L-1)}{2\v L \pi}\\
&+\frac{-\sqrt{-(\v L- \xf)^2+1}+(\xf-\v L)sin^{-1}(\v L-\xf)+\frac{\pi \xf}{2}}{2\v L \pi}\bigg|^{\xf}_{1-\v L}\\
&=\frac{\frac{3 \pi \v L + \pi \xf}{2}+(\xf-\v L)sin^{-1}(\v L-\xf)-\sqrt{1-(\v L-\xf)^2}}{2\v L \pi}\\
\end{split}
\end{equation}

$\xf >\v L+1$
\begin{equation}
\begin{split}
F(\xf)&=\int_{-1-\v L}^{-1+\v L}\frac{sin^{-1}(\xf+\v L)+\frac{\pi}{2}}{2\v L \pi}\,d(\xf)\\
&+\int_{-1+\v L}^{1-\v L}\frac{sin^{-1}(\xf+\v L)-sin^{-1}(\xf-\v L)}{2\v L \pi}\,d(\xf)\\
&+\int_{1-\v L}^{1+\v L}\frac{1}{2\v L \pi}(sin^{-1}(-\xf+\v L)+\frac{\pi}{2})\,d(\xf)\\
&=1\\
\end{split}
\end{equation}

\subsubsection{Statistical distance for fabric position}\label{s:fabric}
%$y=1+\v_{1} L$.
\begin{equation}
\begin{split}
&\Dd(\Xf_{\w_1},\Xf_{\w_2}) = \left| F(\xf_{\w_1|\xf=1+\v_{1}L})-F(\xf_{\w_2|\xf=1+\v_{1}L})\right| =  1\\
&-\frac{\frac{3 \pi \v_{2} L + \pi \xf}{2}+(\xf-\v_{2} L)sin^{-1}(\v_{2} L-\xf)-\sqrt{1-(\v_{2} L-\xf)^2}}{2\v_{2} L \pi}\\
&= 1\\
&-\frac{{3 \pi \v_{2} L + \pi \xf}+2(\xf-\v_{2} L)sin^{-1}(\v_{2} L-\xf)-2\sqrt{1-(\v_{2} L-\xf)^2}}{4\v_{2} L \pi}\\
&=\frac{{\pi \v_{2} L - \pi \xf} - 2(\xf-\v_{2} L)sin^{-1}(\v_{2} L-\xf) + 2\sqrt{1-(\v_{2} L-\xf)^2}}{4\v_{2} L \pi}\\
&=\frac{\pi (\v_{2}L-1-\v_{1}L)  - 2(1 + \v_{1} L - \v_{2} L)sin^{-1}(\v_{2} L- 1 - \v_{1} L )}{4\v_{2} L \pi}\\
&+\frac{2\sqrt{1-(\v_{2} L- 1 - \v_{1} L)^2}}{4\v_{2} L \pi}\\
\end{split}
\end{equation}

\subsection{The proof of $\Dd(\Xf_{\w_1},\Xf_{\w_2})$ increases with $\L$}\label{s:increase}
From \eqref{e:ks:classification},
\begin{equation}
\begin{split}
&\frac{d\Dd(\Xf_{\w_1},\Xf_{\w_2})}{d\L}\\
&=\frac{\pi-2(\sqrt{-\L\dv(\L\dv-2)}+2sin^{-1}(1-\L\dv))}{4\pi\v_{2}\L^2}
\end{split}
\end{equation}

We let $f(\L)=\pi-2(\sqrt{-\L\dv(\L\v-2)}+2sin^{-1}(1-\L\dv))$.
\begin{equation}
\begin{split}
&\frac{df(\L)}{d\L}=\frac{2}{\sqrt{1-(-\L\dv+1)^2}}-\frac{-2\L\dv+2}{\sqrt{-(\L\dv-2)\L\dv}}\\
\end{split}
\end{equation}
We let $\frac{df(\L)}{d\L}=0$, $\min\{f(\L)\}=0$ at $\L=0$.
Therefore, $\frac{d\Dd(\Xf_{\w_1},\Xf_{\w_2})}{d\L}>0, L\in(0,+\infty]$, which indicates $\Dd(\Xf_{\w_1},\Xf_{\w_2})$ is increasing in line with $\L$.

\subsection{The proof of $\Dd(\Xf_{\w_1},\Xf_{\w_2})$ increases with $|\w_{2}-\w_{1}|$}\label{s:fre}
From \eqref{e:ks:classification},
\begin{equation}
\frac{d\Dd(\Xf_{\w_1},\Xf_{\w_2})}{d\dv}=\frac{\pi-2sin^{-1}(1-\L \dv)}{4\pi \v_{2}}
\end{equation}
$\max\{2sin^{-1}(1-\L \dv)\}=\pi$. Therefore $\frac{d\Dd(\Xf_{\w_1},\Xf_{\w_2})}{d\dv}>0$. Therefore, $\Dd(\Xf_{\w_1},\Xf_{\w_2})$ is raising when $\dv$ is increasing.

%when $\v_{2}>\v_{1}$, $\lim\limits_{L\rightarrow 1}\Dd(\Xf_{\w_1},\Xf_{\w_2})>0$.
\subsection{Error estimation of hand-made Scotch yoke mechanism}\label{s:rmse}
This is to compute the time interval of each adjacent lowest position occurred. 
\begin{equation}
	t=|\mathop{\arg\min}_{x}(\xf_{x})-\mathop{\arg\min}_{y}(\xf_{y})|
\end{equation}
Where $t$ is time interval, $\xf_{x}$ and $\xf_{y}$ means the lowest number in one frequency and in the next respectively. 

\ts{not sure whether i need to put it in appendix. because it is respectively short and simple}
